# Supplementary material for: ForeAct: Steering Your VLA with Efficient Visual Foresight Planning
Source: arXiv:2602.12322 source file (2026-02-12)
Supplement: Supplementary file 1 [file supplementary.tex]

% CVPR 2024 Paper Template; see https://github.com/cvpr-org/author-kit

% \documentclass[10pt,twocolumn,letterpaper]{article}

% %%%%%%%%% PAPER TYPE  - PLEASE UPDATE FOR FINAL VERSION
% % \usepackage{cvpr}              % To produce the CAMERA-READY version
% %\usepackage[review]{cvpr}      % To produce the REVIEW version
% \usepackage[pagenumbers]{cvpr} % To force page numbers, e.g. for an arXiv version

% % Import additional packages in the preamble file, before hyperref
% \input{preamble}

% % It is strongly recommended to use hyperref, especially for the review version.
% % hyperref with option pagebackref eases the reviewers' job.
% % Please disable hyperref *only* if you encounter grave issues, 
% % e.g. with the file validation for the camera-ready version.
% %
% % If you comment hyperref and then uncomment it, you should delete *.aux before re-running LaTeX.
% % (Or just hit 'q' on the first LaTeX run, let it finish, and you should be clear).
% \definecolor{cvprblue}{rgb}{0.21,0.49,0.74}
% \usepackage[pagebackref,breaklinks,colorlinks,citecolor=cvprblue]{hyperref}
% \usepackage{subcaption}
% \usepackage{multirow}

% %%%%%%%%% PAPER ID  - PLEASE UPDATE
% \def\paperID{4742} % *** Enter the Paper ID here
% \def\confName{CVPR}
% \def\confYear{2024}
% \input{pacakges}
% \input{macros}
% \input{math_commands}

\documentclass[10pt,twocolumn,letterpaper]{article}

%%%%%%%%% PAPER TYPE  - PLEASE UPDATE FOR FINAL VERSION
% \usepackage{cvpr}              % To produce the CAMERA-READY version
\usepackage[review]{cvpr}      % To produce the REVIEW version
% \usepackage[pagenumbers]{cvpr} % To force page numbers, e.g. for an arXiv version

% Import additional packages in the preamble file, before hyperref
\input{preamble}

% It is strongly recommended to use hyperref, especially for the review version.
% hyperref with option pagebackref eases the reviewers' job.
% Please disable hyperref *only* if you encounter grave issues, 
% e.g. with the file validation for the camera-ready version.
%
% If you comment hyperref and then uncomment it, you should delete *.aux before re-running LaTeX.
% (Or just hit 'q' on the first LaTeX run, let it finish, and you should be clear).
\definecolor{cvprblue}{rgb}{0.21,0.49,0.74}
\usepackage[pagebackref,breaklinks,colorlinks,allcolors=cvprblue,citecolor=cvprblue]{hyperref}

%%%%%%%%% PAPER ID  - PLEASE UPDATE
 % *** Enter the Paper ID here

\input{pacakges}
\input{macros}
\input{math_commands}

%%%%%%%%% TITLE - PLEASE UPDATE
\title{Plan, Imagine, then Act: Steering Your VLA with Efficient Visually Grounded Planning ---- Supplementary Materials}

%%%%%%%%% AUTHORS - PLEASE UPDATE

\setcounter{section}{-1}
\begin{document}

\maketitle
\input{sec/X_suppl}

% \newpage

% %\section*{Acknowledgments}
% %We would like to thank Google Cloud and Lambda Labs for their invaluable support in providing computing resources.

% {
%     \small
%     \bibliographystyle{ieeenat_fullname}
%     \bibliography{main}
% }

% WARNING: do not forget to delete the supplementary pages from your submission 
% \input{sec/X_suppl}

\end{document}
